# Supplementary material for: Can Autonomous Vehicles Identify, Recover From, and Adapt to Distribution Shifts?
Source: arXiv:2006.14911 source file (2020-09-02)
Supplement: Supplementary file 1 [file supp.pdf]

## References


Akkaya, I., Andrychowicz, M., Chociej, M., Litwin, M., McGrew, B., Petron, A., Paino, A., Plappert, M., Powell, G., Ribas, R., et al. Solving Rubik's cube with a robot hand. *arXiv preprint arXiv:1910.07113*, 2019.

Amodei, D., Olah, C., Steinhardt, J., Christiano, P., Schulman, J., and Mané, D. Concrete problems in AI safety. *arXiv preprint arXiv:1606.06565*, 2016.

Barber, D. *Bayesian reasoning and machine learning*. Cambridge University Press, 2012.

Bellman, R. E. *Adaptive control processes: a guided tour*. Princeton university press, 2015.

Bishop, C. M. Mixture density networks. 1994.

Blundell, C., Cornebise, J., Kavukcuoglu, K., and Wierstra, D. Weight uncertainty in neural networks. *arXiv preprint arXiv:1505.05424*, 2015.

Caesar, H., Bankiti, V., Lang, A. H., Vora, S., Liong, V. E., Xu, Q., Krishnan, A., Pan, Y., Baldan, G., and Beijbom, O. nuscenes: A multimodal dataset for autonomous driving. *arXiv preprint arXiv:1903.11027*, 2019.

Castro, P. S. and Precup, D. Using bisimulation for policy transfer in MDPs. In *AAAI Conference on Artificial Intelligence*, 2010.

Cesa-Bianchi, N. and Lugosi, G. *Prediction, learning, and games*. Cambridge University Press, 2006.

Chai, Y., Sapp, B., Bansal, M., and Anguelov, D. Multipath: Multiple probabilistic anchor trajectory hypotheses for behavior prediction. *arXiv preprint arXiv:1910.05449*, 2019.

Chen, D., Zhou, B., Koltun, V., and Krähenbühl, P. Learning by cheating. *arXiv preprint arXiv:1912.12294*, 2019.

Christiano, P. F., Leike, J., Brown, T., Martic, M., Legg, S., and Amodei, D. Deep reinforcement learning from human preferences. In *Advances in Neural Information Processing Systems*, pp. 4299–4307, 2017.

Chua, K., Calandra, R., McAllister, R., and Levine, S. Deep reinforcement learning in a handful of trials using probabilistic dynamics models. In *Neural Information Processing Systems (NeurIPS)*, pp. 4754–4765, 2018.

Codevilla, F., Miiller, M., López, A., Koltun, V., and Dosovitskiy, A. End-to-end driving via conditional imitation learning. In *International Conference on Robotics and Automation (ICRA)*, pp. 1–9. IEEE, 2018.

Codevilla, F., Santana, E., López, A. M., and Gaidon, A. Exploring the limitations of behavior cloning for autonomous driving. In *International Conference on Computer Vision (ICCV)*, pp. 9329–9338, 2019.

Coley, G., Wesley, A., Reed, N., and Parry, I. Driver reaction times to familiar, but unexpected events. *TRL Published Project Report*, 2009.

Cronrath, C., Jorge, E., Moberg, J., Jirstrand, M., and Lennartson, B. BAgger: A Bayesian algorithm for safe and query-efficient imitation learning. https://personalrobotics.cs.washington.edu/workshops/mlmp2018/assets/docs/24_CameraReadySubmission_180928_BAgger.pdf, 2018.

Cui, H., Radosavljevic, V., Chou, F.-C., Lin, T.-H., Nguyen, T., Huang, T.-K., Schneider, J., and Djuric, N. Multimodal trajectory predictions for autonomous driving using deep convolutional networks. In *2019 International Conference on Robotics and Automation (ICRA)*, pp. 2090–2096. IEEE, 2019.

de Haan, P., Jayaraman, D., and Levine, S. Causal confusion in imitation learning. In *Neural Information Processing Systems (NeurIPS)*, pp. 11693–11704, 2019.

Dosovitskiy, A., Ros, G., Codevilla, F., Lopez, A., and Koltun, V. CARLA: An open urban driving simulator. *arXiv preprint arXiv:1711.03938*, 2017.

Du, Y., Lin, T., and Mordatch, I. Model based planning with energy based models. *arXiv preprint arXiv:1909.06878*, 2019.

Embrechts, P., Klüppelberg, C., and Mikosch, T. *Modelling extremal events: for insurance and finance*, volume 33. Springer Science & Business Media, 2013.

Finn, C., Abbeel, P., and Levine, S. Model-agnostic metalearning for fast adaptation of deep networks. In *International Conference on Machine Learning (ICML)*, pp. 1126–1135, 2017.

French, R. M. Catastrophic forgetting in connectionist networks. *Trends in cognitive sciences*, 3(4):128–135, 1999.

Gal, Y. and Ghahramani, Z. Dropout as a Bayesian approximation: Representing model uncertainty in deep learning. In *International Conference on Machine Learning (ICML)*, pp. 1050–1059, 2016.

Graves, A. Practical variational inference for neural networks. In *Neural Information Processing Systems (NeurIPS)*, pp. 2348–2356, 2011.

Hernández-Lobato, J. M. and Adams, R. Probabilistic backpropagation for scalable learning of Bayesian neural networks. In *International Conference on Machine Learning (ICML)*, pp. 1861–1869, 2015.

Kahn, G., Villaflor, A., Pong, V., Abbeel, P., and Levine, S. Uncertainty-aware reinforcement learning for collision avoidance. *arXiv preprint arXiv:1702.01182*, 2017.

Kenton, Z., Filos, A., Evans, O., and Gal, Y. Generalizing from a few environments in safety-critical reinforcement learning. *arXiv preprint arXiv:1907.01475*, 2019.

Kesten, R., Usman, M., Houston, J., Pandya, T., Nadhamuni, K., Ferreira, A., Yuan, M., Low, B., Jain, A., Ondruska, P., Omari, S., Shah, S., Kulkarni, A., Kazakova, A., Tao, C., Platinsky, L., Jiang, W., and Shet, V. Lyft level 5 av dataset 2019, 2019. URL https://level5.lyft.com/dataset/.

Kingma, D. P. and Ba, J. Adam: A method for stochastic optimization. *arXiv preprint arXiv:1412.6980*, 2014.

Lakshminarayanan, B., Pritzel, A., and Blundell, C. Simple and scalable predictive uncertainty estimation using deep ensembles. In *Neural Information Processing Systems (NeurIPS)*, pp. 6402–6413, 2017.

Leike, J., Martic, M., Krakovna, V., Ortega, P. A., Everitt, T., Lefrancq, A., Orseau, L., and Legg, S. AI safety gridworlds. *arXiv preprint arXiv:1711.09883*, 2017.

Li, Z., Motoyoshi, T., Sasaki, K., Ogata, T., and Sugano, S. Rethinking self-driving: Multi-task knowledge for better generalization and accident explanation ability. *arXiv preprint arXiv:1809.11100*, 2018.

Liang, X., Wang, T., Yang, L., and Xing, E. Cirl: Controllable imitative reinforcement learning for vision-based self-driving. In *European Conference on Computer Vision (ECCV)*, pp. 584–599, 2018.

Liu, C. and Atkeson, C. G. Standing balance control using a trajectory library. In *2009 IEEE/RSJ International Conference on Intelligent Robots and Systems*, pp. 3031–3036. IEEE, 2009.

McAllister, R., Kahn, G., Clune, J., and Levine, S. Robustness to out-of-distribution inputs via task-aware generative uncertainty. In *International Conference on Robotics and Automation (ICRA)*, pp. 2083–2089. IEEE, 2019.

Michelmore, R., Kwiatkowska, M., and Gal, Y. Evaluating uncertainty quantification in end-to-end autonomous driving control. *arXiv preprint arXiv:1811.06817*, 2018.

National Highway Traffic Safety Administration. Pre-crash scenario typology for crash avoidance research, 2007. URL https://www.nhtsa.gov/sites/nhtsa.dot.gov/files/pre-crash_scenario_typology-final_pdf_version_5-2-07.pdf.

Neal, R. M. *Bayesian learning for neural networks*, volume 118. Springer Science & Business Media, 2012.

OpenAI, M. A., Baker, B., Chociej, M., Józefowicz, R., McGrew, B., Pachocki, J., Petron, A., Plappert, M., Powell, G., Ray, A., et al. Learning dexterous in-hand manipulation. *arXiv preprint arXiv:1808.00177*, 2018.

Phan-Minh, T., Grigore, E. C., Boulton, F. A., Beijbom, O., and Wolff, E. M. Covernet: Multimodal behavior prediction using trajectory sets. *arXiv preprint arXiv:1911.10298*, 2019.

Pomerleau, D. A. Alvinn: An autonomous land vehicle in a neural network. In *Neural Information Processing Systems (NeurIPS)*, pp. 305–313, 1989.

Quionero-Candela, J., Sugiyama, M., Schwaighofer, A., and Lawrence, N. D. *Dataset shift in machine learning*. MIT Press, 2009.

Rajeswaran, A., Ghotra, S., Ravindran, B., and Levine, S. Epopt: Learning robust neural network policies using model ensembles. *arXiv preprint arXiv:1610.01283*, 2016.

Rezende, D. J. and Mohamed, S. Variational inference with normalizing flows. *arXiv preprint arXiv:1505.05770*, 2015.

Rhinehart, N., Kitani, K. M., and Vernaza, P. R2P2: A reparameterized pushforward policy for diverse, precise generative path forecasting. In *European Conference on Computer Vision (ECCV)*, pp. 772–788, 2018.

Rhinehart, N., McAllister, R., Kitani, K., and Levine, S. PRECOG: Prediction conditioned on goals in visual multi-agent settings. *International Conference on Computer Vision*, 2019.

Rhinehart, N., McAllister, R., and Levine, S. Deep imitative models for flexible inference, planning, and control. In *International Conference on Learning Representations (ICLR)*, April 2020.

Ros, G., Koltun, V., Codevilla, F., and Lopez, M. A. CARLA challenge, 2019. URL https://carlachallenge.org.

Ross, S., Gordon, G., and Bagnell, D. A reduction of imitation learning and structured prediction to no-regret online learning. In *Artificial Intelligence and Statistics (AISTATS)*, pp. 627–635, 2011.

Sadeghi, F. and Levine, S. Cad2rl: Real single-image flight without a single real image. *arXiv preprint arXiv:1611.04201*, 2016.

Sauer, A., Savinov, N., and Geiger, A. Conditional affordance learning for driving in urban environments. *arXiv preprint arXiv:1806.06498*, 2018.

Snoek, J., Ovadia, Y., Fertig, E., Lakshminarayanan, B., Nowozin, S., Sculley, D., Dillon, J., Ren, J., and Nado, Z. Can you trust your model's uncertainty? evaluating predictive uncertainty under dataset shift. In *Neural Information Processing Systems (NeurIPS)*, pp. 13969–13980, 2019.

Sugiyama, M. and Kawanabe, M. *Machine learning in non-stationary environments: Introduction to covariate shift adaptation*. MIT press, 2012.

Sun, P., Kretzschmar, H., Dotiwalla, X., Chouard, A., Patnaik, V., Tsui, P., Guo, J., Zhou, Y., Chai, Y., Caine, B., et al. Scalability in perception for autonomous driving: An open dataset benchmark. *arXiv preprint arXiv:1912.04838*, 2019.

Tang, Y. C., Zhang, J., and Salakhutdinov, R. Worst cases policy gradients. *arXiv preprint arXiv:1911.03618*, 2019.

Taoka, G. T. Brake reaction times of unalerted drivers. *ITE journal*, 59(3):19–21, 1989.

Uria, B., Côté, M.-A., Gregor, K., Murray, I., and Larochelle, H. Neural autoregressive distribution estimation. *The Journal of Machine Learning Research*, 17 (1):7184–7220, 2016.

Wald, A. Contributions to the theory of statistical estimation and testing hypotheses. *The Annals of Mathematical Statistics*, 10(4):299–326, 1939.

Widrow, B. and Smith, F. W. Pattern-recognizing control systems, 1964.

Zhang, J. and Cho, K. Query-efficient imitation learning for end-to-end autonomous driving. *arXiv preprint arXiv:1605.06450*, 2016.

Zhou, A., Jang, E., Kappler, D., Herzog, A., Khansari, M., Wohlhart, P., Bai, Y., Kalakrishnan, M., Levine, S., and Finn, C. Watch, try, learn: Meta-learning from demonstrations and reward. *arXiv preprint arXiv:1906.03352*, 2019.

## A. CARNOVEL: Suite of Tasks Under Distribution Shift

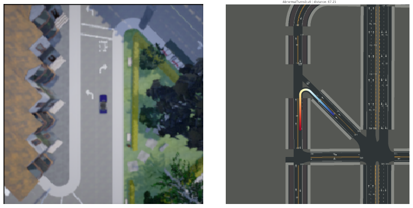
(a) AbnormalTurns0-v0

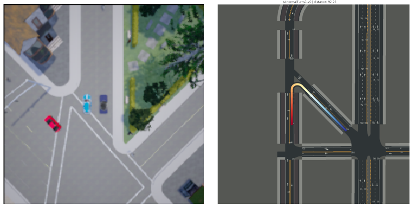
(b) AbnormalTurns1-v0

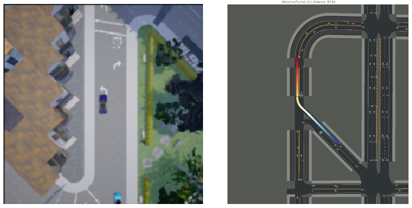
(c) AbnormalTurns2-v0

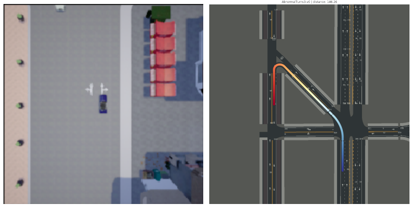
(d) AbnormalTurns3-v0

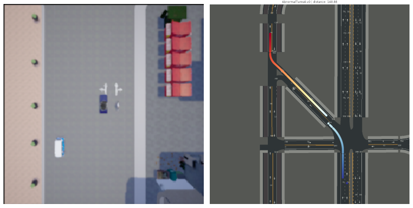
(e) AbnormalTurns4-v0

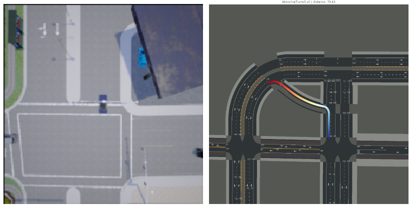
(f) AbnormalTurns5-v0

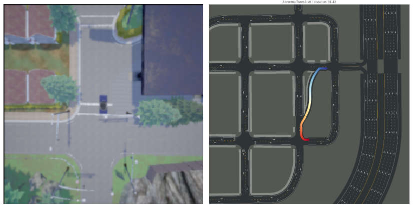
(g) AbnormalTurns6-v0

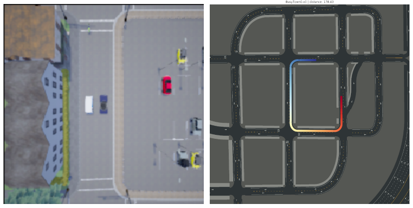
(h) BusyTown0-v0

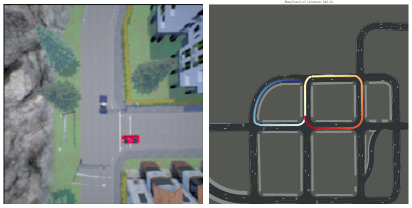
(i) BusyTown1-v0

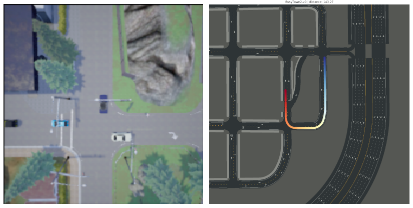
(j) BusyTown2-v0

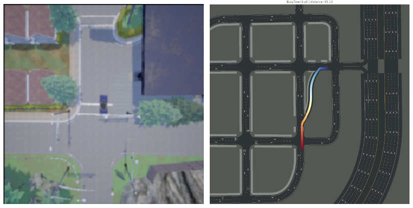
(k) BusyTown3-v0

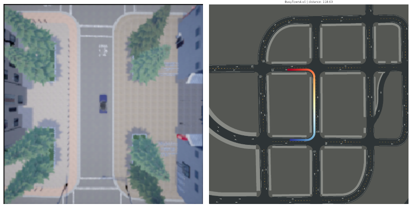
(l) BusyTown4-v0

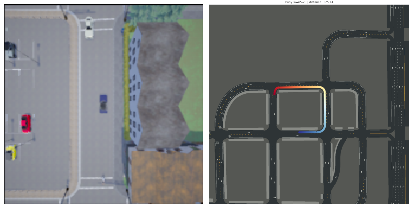
(m) BusyTown5-v0

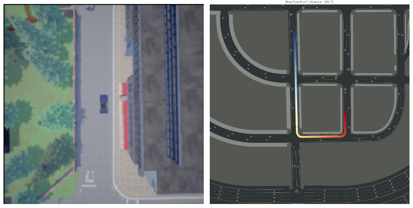
(n) BusyTown6-v0

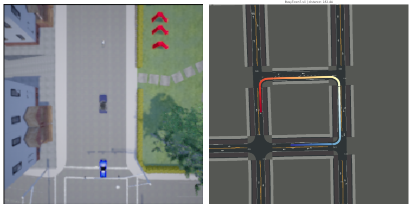
(o) BusyTown7-v0

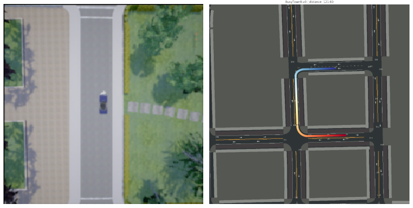

(p) BusyTown8-v0

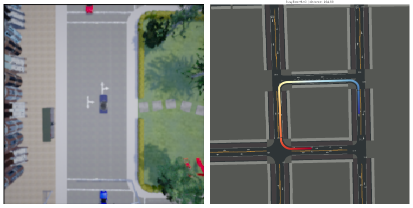

(q) BusyTown9-v0

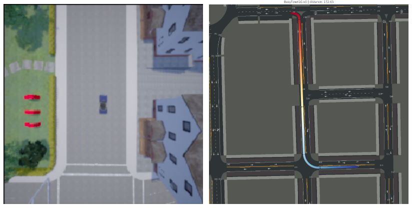

(r) BusyTown10-v0

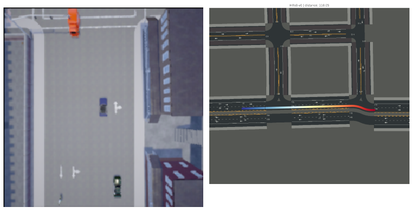

(s) Hills0-v0

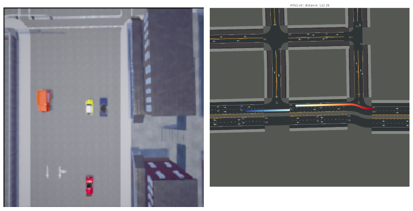

(t) Hills1-v0

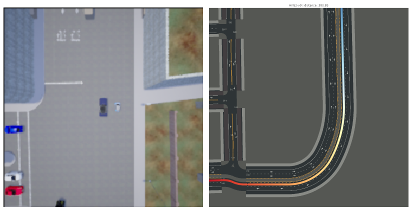

(u) Hills2-v0

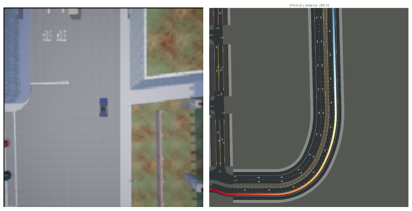

(v) Hills3-v0

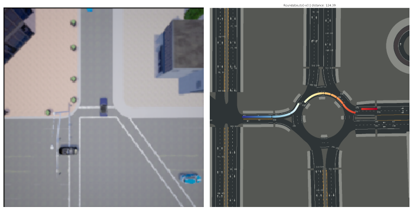

(w) Roundabouts0-v0

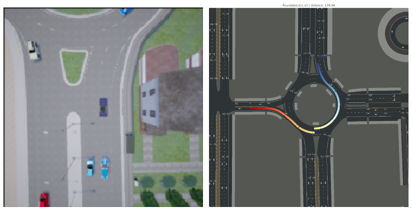

(x) Roundabouts1-v0

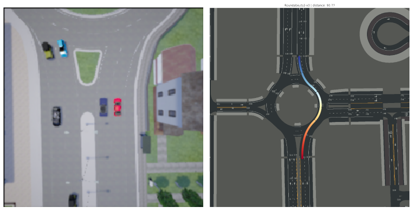

(y) Roundabouts2-v0

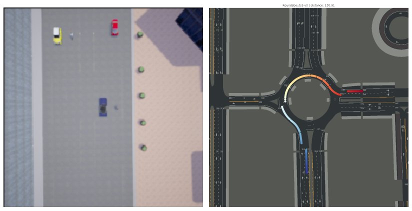

(z) Roundabouts3-v0

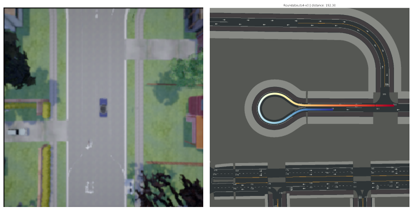

(aa) Roundabouts4-v0

## B. Experimental Results on CARNOVEL

*Table 4.* We evaluate different autonomous driving methods in terms of their robustness to distribution shifts, in our new benchmark, CARNOVEL. All methods are trained on CARLA Town01 using imitation learning on expert demonstrations from the autopilot (Dosovitskiy et al., 2017). A "†" indicates methods that use first-person camera view, as in (Chen et al., 2019), a "♣" methods that use LIDAR observation, as in (Rhinehart et al., 2020) and a "◇" methods that use the ground truth game engine state, as in (Chen et al., 2019). A "★" indicates that we used the reference implementation from the original paper, otherwise we used our implementation. For all the scenes we chose pairs of start-destination locations and ran 10 trials with randomized initial simulator state for each pair. Standard errors are in gray (via bootstrap sampling). The **outperforming** method is in bold.

| | AbnormalTurns | | | BusyTown | | |
|---|---|---|---|---|---|---|
| **Methods** | Success ↑ (7 × 10 scenes, %) | Infra/km ↓ ($\times 1e{-}3$) | Distance ↑ (m) | Success ↑ (11 × 10 scenes, %) | Infra/km ↓ ($\times 1e{-}3$) | Distance ↑ (m) |
| CIL♣★ (Codevilla et al., 2018) | 65.71±07.37 | 07.04±05.07 | 128±020 | 05.45±06.35 | 11.49±03.66 | 217±033 |
| LbC†★ (Chen et al., 2019) | 00.00±00.00 | 05.81±00.58 | 208±004 | 20.00±13.48 | 03.96±00.15 | 374±016 |
| LbC-GT◇★ (Chen et al., 2019) | 02.86±06.39 | **03.68**±00.34 | 217±033 | 65.45±07.60 | 02.59±00.02 | 400±006 |
| DIM♣ (Rhinehart et al., 2020) | 74.28±11.26 | 05.56±04.06 | 108±017 | 47.13±14.54 | 08.47±05.22 | 175±026 |
| RIP-BCM♣ (baseline, cf. Table 1) | 68.57±09.03 | 07.93±03.73 | 096±017 | 50.90±20.64 | 03.74±05.52 | 175±031 |
| RIP-MA♣ (ours, cf. Section 3.3.2) | **84.28**±14.20 | 07.86±05.70 | 102±015 | **64.54±23.25** | 05.86±03.99 | 170±033 |
| RIP-WCM♣ (ours, cf. Section 3.3.1) | **87.14**±14.20 | **04.91**±03.60 | 102±021 | **62.72**±05.16 | **03.17**±02.04 | 167±021 |

| | Hills | | | Roundabouts | | |
|---|---|---|---|---|---|---|
| **Methods** | Success ↑ (4 × 10 scenes, %) | Infra/km ↓ ($\times 1e{-}3$) | Distance ↑ (m) | Success ↑ (5 × 10 scenes, %) | Infra/km ↓ ($\times 1e{-}3$) | Distance ↑ (m) |
| CIL♣★ (Codevilla et al., 2018) | 60.00±29.34 | 04.74±03.02 | 219±034 | 20.00±00.00 | **03.60**±03.23 | 269±021 |
| LbC†★ (Chen et al., 2019) | 50.00±00.00 | 01.61±00.15 | 541±101 | 08.00±10.95 | 03.70±00.72 | 323±043 |
| LbC-GT◇★ (Chen et al., 2019) | 05.00±11.18 | 03.36±00.26 | 312±020 | 00.00±00.00 | 06.47±00.99 | 123±018 |
| DIM♣ (Rhinehart et al., 2020) | 70.00±10.54 | 06.87±04.09 | 195±012 | 20.00±09.42 | 06.19±04.73 | 240±044 |
| RIP-BCM♣ (baseline, cf. Table 1) | 75.00±00.00 | 05.49±04.03 | 191±013 | 06.00±09.66 | 06.78±07.05 | 251±027 |
| RIP-MA♣ (ours, cf. Section 3.3.2) | **97.50**±07.90 | **00.26**±00.54 | 196±013 | **38.00**±06.32 | 05.48±05.56 | 271±047 |
| RIP-WCM♣ (ours, cf. Section 3.3.1) | **87.50**±13.17 | **01.83**±01.73 | 191±006 | **42.00**±06.32 | 04.32±01.91 | 217±030 |

## C. AdaRIP Examples

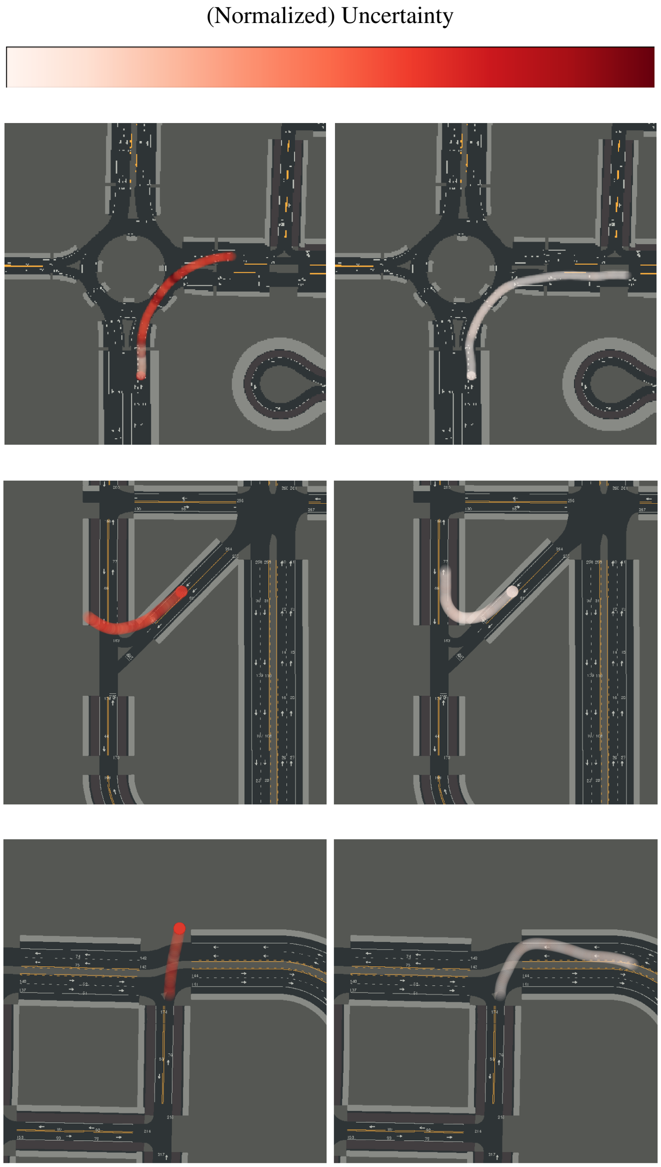


(a) RIP (b) AdaRIP

*Figure 8.* Examples where the non-adaptive method (a) fails to recover from a distribution shift, despite it being able to detect it. The adaptive method (b) queries the human driver when uncertain (dark red), then uses the online demonstrations for updating its model, resulting into confident (light red, white) and safe trajectories.

## D. Online Planning with a Trajectory Library

In the absence of scalable global optimizers, we search the trajectory space in Eqn. (4) by restricting the search space to a trajectory library (Liu & Atkeson, 2009), $\mathcal{T}_{\mathbf{Y}}$, a finite set of fixed trajectories. In this work, we perform $K$-means clustering of the expert plan's from the training distribution and keep $64$ of the centroids, as illustrated in Figure 9. Therefore we efficiently solve a search problem over a discrete space rather than an optimization problem of continuous variables. The modified objective is:

$$\mathbf{y}^{\mathcal{G}}_{\text{RIP}} \approx \underset{\mathbf{y} \in \mathcal{T}_{\mathbf{Y}}}{\arg\max} \bigoplus_{\boldsymbol{\theta} \in \text{supp}\left(p(\boldsymbol{\theta}|\mathcal{D})\right)} \log p(\mathbf{y}|\mathcal{G}, \mathbf{x}; \boldsymbol{\theta}) \tag{10}$$

Solving for Eqn. (10) results in $\times 20$ improvement in runtime compared to the gradient descent alternative. Although in in-distribution scenes solving Eqn. (10) over Eqn. (4) does not deteriorate perfomance, in out-of-distribution scenes the trajectory library, $\mathcal{T}_{\mathbf{Y}}$, is not useful. Therefore in the experiments (c.f. Section 4.2.3) we used online gradient-descent. Future work lies in developing a hybrid optimization method that takes advantage of the speedup the trajectory library provides without a decrease in performance in out-of-distribution scenarios.

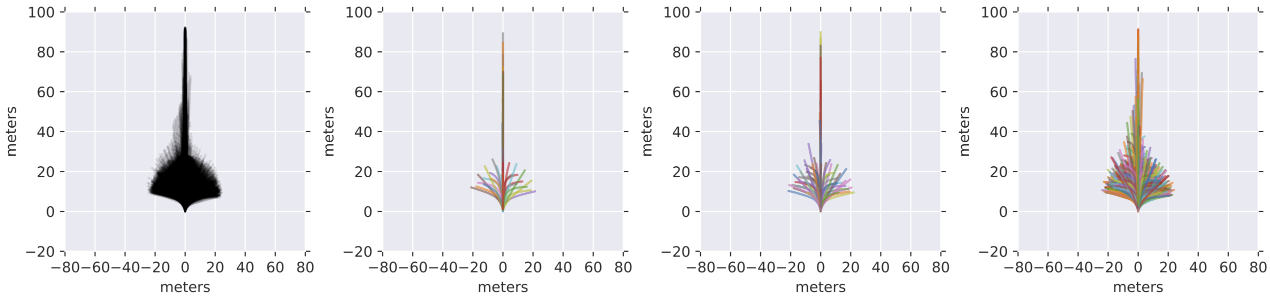


(a) Trajectories (b) $K = 64$ (c) $K = 128$ (d) $K = 1024$

*Figure 9.* Our trajectory library from CARLA's autopilot demonstrations, 4 seconds.
